# Supplementary material for: Many-body theory of false vacuum decay in quantum spin chains
Source: arXiv:2508.13780 source file (2026-09-19)
Supplement: Supplementary file 1 [file Supplementary.tex]

\documentclass[aps, pra, onecolumn, superscriptaddress]{revtex4-2}

\usepackage{amssymb, amsmath, amsthm}
\usepackage[utf8]{inputenc}
\usepackage[english]{babel}
\usepackage{color}
\usepackage{graphicx}
\usepackage{hyperref}
\usepackage{bm}
\usepackage{physics}
\usepackage{dsfont}
\usepackage[normalem]{ulem}
\usepackage{xcolor}
\usepackage[capitalize]{cleveref}

\begin{document}
% ======================
% Supplementary Material
% ======================

\onecolumngrid
\clearpage

\title{Supplementary material\\
Many-body theory of false vacuum decay in quantum spin chains
}

\author{Christian Johansen}
\email{christianhoj.johansen@ino.cnr.it}
\affiliation{Pitaevskii BEC Center, CNR-INO and Dipartimento di Fisica, Università di Trento, Trento, Italy}
\author{Alessio Recati}
\email{alessio.recati@cnr.it}
\affiliation{Pitaevskii BEC Center, CNR-INO and Dipartimento di Fisica, Università di Trento, Trento, Italy}
\affiliation{INFN-TIFPA, Trento Institute for Fundamental Physics and Applications, I-38123 Trento, Italy}
\author{Iacopo Carusotto}
\email{iacopo.carusotto@ino.cnr.it}
\affiliation{Pitaevskii BEC Center, CNR-INO and Dipartimento di Fisica, Università di Trento, Trento, Italy}
\affiliation{INFN-TIFPA, Trento Institute for Fundamental Physics and Applications, I-38123 Trento, Italy}
\author{Alberto Biella}
\email{alberto.biella@cnr.it}
\affiliation{Pitaevskii BEC Center, CNR-INO and Dipartimento di Fisica, Università di Trento, Trento, Italy}
\affiliation{INFN-TIFPA, Trento Institute for Fundamental Physics and Applications, I-38123 Trento, Italy}
  \date{\today}
  \maketitle
\setcounter{equation}{0}
\setcounter{figure}{0}
\setcounter{table}{0}
\setcounter{page}{1}
\makeatletter
\renewcommand{\theequation}{S\arabic{equation}}
\renewcommand{\thefigure}{S\arabic{figure}}
\renewcommand{\bibnumfmt}[1]{[S#1]}
\renewcommand{\citenumfont}[1]{S#1}

In this supplementary material we will derive the Coherent Boson Theory (CBT) starting from the transverse-field Ising model. In \cref{sec:sys} we briefly discuss the mapping of the spin Hamiltonian to a fermion model. Following this, \cref{sec:two_fermion} summarizes the two fermion states. These first two section closely follow the work in \cite{Rutkevich1999}, but are included here to give a self-consistent representation. 
Using the results from the previous section we then develop the CBT in \cref{sec:CBT}. 
\section{Thermodynamic limit and fermion mapping}\label{sec:sys}
We consider one-dimensional chain with $N$ sites.
The Hamiltonian under consideration is the transverse-field Ising model quenched by a weak longitudinal field
\begin{equation}
    H(t)=-J\left(\sum_{n=1}^{N-1}\sigma^x_n\sigma^x_{n+1}+h_\perp \sum_{n=1}^N\sigma^z_n+\theta(t)h_\parallel\sum_{n=1}^N\sigma^x_n,\right),
\end{equation}
where $\theta(t)$ is the Heaviside function.
Prior to the quench, the system is diagonalized by a Jordan-Wigner transformation followed by a Fourier and a Bogoliubov transformation \cite{IsingBeginners}. 
The diagonalized prequench Hamiltonian takes the form
\begin{equation}\label{eq:H_t0}
H(t<0)=\sum_{k}\epsilon_k \tilde{\gamma}_k^\dagger\tilde{\gamma}_k,
\end{equation}
where $k\in\{\pm \frac{(2n-1)\pi}{N},\,n=1,...,N/2\}$ and $\tilde{\gamma}_k$ is a fermionic annihilation operator, while $\epsilon_k$ is the dispersion relation given by
\begin{equation}\label{eq:HTFIM_disp}
    \epsilon_k=2J \sqrt{1 - 2 h_\perp  \cos(k) + h_\perp^2}.
\end{equation}
The annihilation operators obey the fermionic anti-commutation relations
\begin{equation}\label{eq:fermionAC_finite}
    \{\tilde{\gamma}_q,\tilde{\gamma}_k\}=\{\tilde{\gamma}_q^\dagger,\tilde{\gamma}_k^\dagger\}=0,\quad \{\tilde{\gamma}_k,\tilde{\gamma}_q^\dagger\}=\delta_{q,k}.
\end{equation} 
The ground state of the prequenched system is two-fold degenerate (for $h_\perp<J$) and leads to a spontaneous symmetry breaking with the spins having a projection onto the longitudinal axis of either $\pm M=\pm\left(1-h_\perp^2\right)^{1/8}$.
The excitations represented by the $\gamma_k^\dagger$ correspond to the creation of a delocalized kink \cite{IsingBeginners}. 
The width of the delocalized kink, in units of the lattice distance, can be approximated as \cite{WidthHeyl2020} 
\begin{equation}\label{eq:W}
W\approx\frac{\sqrt{h_\perp}}{1-h_\perp}
\end{equation}

Considering the thermodynamic limit, the momentum spacing ($\Delta_k$) becomes infinitesimal and thus leads to the following relations
\begin{equation}
    \begin{aligned}
        \delta_{n\%N}=&\lim_{N\to\infty}\frac{1}{N}\sum_ke^{ikn}=\int_{-\pi}^\pi\frac{d\theta}{2\pi}e^{i\theta n},\\
        \lim_{N\to\infty}\frac{\delta_k}{\Delta_k}=&\delta(\theta)=\lim_{N\to\infty}\frac{1}{\Delta_k N}\sum_ne^{i\theta n}, \\
        \lim_{N\to\infty}\frac{1}{\Delta_k}=&\delta(0),\\
        \Delta_k=&\frac{2\pi}{N}.
    \end{aligned}
\end{equation}
For a more streamlined notation the periodic nature of the discrete Kronecker delta will not be written explicitly.
In the thermodynamic limit the $\tilde{\gamma}'s$ obey the anti-commutation relations
\begin{equation}
    \{\tilde{\gamma}(\theta),\tilde{\gamma}^\dagger(\theta')\}=\Delta_k\delta(\theta-\theta'),
\end{equation}
while the Hamiltonian in \cref{eq:H_t0} takes the form
\begin{equation}
    \lim_{N\to\infty}H(t<0)=\int_{-\pi}^\pi \frac{d\theta}{\Delta_k}\epsilon(\theta) \tilde{\gamma}^\dagger(\theta)\tilde{\gamma}(\theta),
\end{equation}
where $\epsilon(\theta)$ is functionally identical to \cref{eq:HTFIM_disp}. 
To find an explicitly $N$-independent form of $H(t<0)$, one can introduce rescaled operators: $\gamma(\theta)=\sqrt{N}\tilde{\gamma}(\theta)$. 
In these operators the Hamiltonian takes the form 
\begin{equation}
    \lim_{N\to\infty}H(t<0)=\int_{-\pi}^\pi \frac{d\theta}{2\pi}\epsilon(\theta) \gamma^\dagger(\theta)\gamma(\theta),
\end{equation}
and the operators obey the anti-commutation relations
\begin{equation}
    \left\{\gamma(\theta),\gamma(\phi)\right\}=N\left\{\tilde{\gamma}(\theta),\tilde{\gamma}(\phi)\right\}=2\pi\delta(\theta-\phi).
\end{equation}
The corresponding real-space operators are 
\begin{equation}
    b_n=\frac{1}{N}\int_{-\pi}^\pi \frac{d\theta}{\Delta_k}e^{-i\theta n}\gamma(\theta)=\int_{-\pi}^\pi \frac{d\theta}{2\pi} e^{-i\theta n}\gamma(\theta),
\end{equation}
and obey the anti-commutation relations
\begin{equation}
    \left\{\tilde{b}_n,\tilde{b}^\dagger_m\right\}=\delta_{n,m}.
\end{equation}
Due to the finite lattice spacing the the inverse Fourier transformation remains discrete
\begin{equation}
        \gamma(\theta)=\sum_{n=1}^N e^{in\theta}b_n.
\end{equation}
In the thermodynamic limit the quenched Hamiltonian can also be written in the fermion basis \cite{Rutkevich1999}
\begin{equation}
    H(t>0)=H(t<0)+V
\end{equation}
with 
\begin{equation}
    V=J\abs{h_\parallel} M \sum_{n=1}^N:\exp\left(-\sum_{j<n}^N\psi^{(+)}_j\psi_j^{(-)}\right):,
\end{equation}
where $:\mathcal{O}:$ symbolizes normal-ordering and 
\begin{equation}
\begin{aligned}
    \psi^{(+)}_j&=i\int_{-\pi}^\pi\frac{d\theta}{\sqrt{ 2\pi}}\frac{e^{ij\theta}}{\sqrt{\epsilon(\theta)}}\left[\gamma(\theta)+\gamma^\dagger(-\theta)\right],\;
    \psi^{(-)}_j=i\int_{-\pi}^\pi\frac{d\theta}{\sqrt{ 2\pi}}e^{ij\theta}\sqrt{\epsilon(\theta)}\left[-\gamma(\theta)+\gamma^\dagger(-\theta)\right].
\end{aligned}
\end{equation}

One can split $V$ into two contributions: one that conserves the kink number $V_0$ and the rest which couples sectors with different number of kinks. 
The simplest way of achieving this is to define $V_0$ in the flat-dispersion limit \cite{Rutkevich1999}
\begin{equation}
    V_0=\lim_{h_\perp\to0}V=J\abs{h_\parallel} M \sum_{n=1}^N:\exp\left(-2\sum_{j<n}^N b^\dagger_jb_j\right):.
\end{equation}
One can thus reorder the quenched Hamiltonian into the form
\begin{equation}
    H(t>0)=H_0+\tilde{V},
\end{equation}
where $H_0=H(t<0)+V_0$ and $\tilde{V}=V-V_0$. 
As $V_0$ does not couple different kink sectors, coupling between sectors with different fermion number is fully described by $V$. 
One notices that since this is normal-ordered exponential of an even number of $\gamma$'s, $V$ can only add or remove an even number of fermions. 
Considering quenches from $\ket{0_+}$ means that for $t<0$ there are no fermions in the system and for $t>0$ one will thus only find states with an even number of fermions. 

\section{Two-fermion states}\label{sec:two_fermion}
If one considers either small longitudinal field or small transverse field, then $\tilde{V}$ only weakly couples sectors with different fermion numbers.
This creates a time scale where the system can be approximated by a truncated Hilbert space consisting of the ground state and a single two-fermion state. 
The two-fermion states has to conserve momentum and we can thus describe the $l$'th two-fermion state as 
\begin{equation}
    \ket{\phi_L}=\mathcal{N}\int_{-\pi}^\pi d\theta\phi_L(\theta)\gamma^\dagger(\theta)\gamma^\dagger(-\theta)\ket{0_+}.
\end{equation}
These states are eigenstates of the two-body problem
with eigenenergies $E_L$
\begin{equation}
    H_0 \ket{\phi_L}=E_L\ket{\phi_L}.
\end{equation}
The normalization $\mathcal{N}$ is defined through the overlap
\begin{equation}
    \braket{\phi_L}{\phi_{L'}}=\mathcal{N}^2\int_{-\pi}^\pi d\theta \,d\phi\,\phi_L^*(\theta)\phi_{L'}(\phi)\bra{0_+}\mathcal{M}_\gamma(\theta,\phi)\ket{0_+}=1.
\end{equation}
The operator product 
\begin{equation}
    \mathcal{M}_\gamma(\theta,\phi)=\gamma(-\theta)\gamma(\theta)\gamma^\dagger(\phi)\gamma^\dagger(-\phi)
\end{equation}
inside the FV expectation value will be important again later so we therefore normal-order it here.
\begin{equation}\label{eq:Mgamma}
\begin{aligned}
    \mathcal{M}_\gamma&=\gamma(-\theta)\left[N\Delta_k\delta(\theta-\phi)-\gamma^\dagger(\phi)\gamma(\theta)\right]\gamma^\dagger(-\phi),\\
    &\;\begin{aligned}
        =(N\Delta_k^2)\delta(\theta-\phi)^2-N\Delta_k\delta(\theta-\phi)\gamma^\dagger(-\phi)\gamma(-\theta)-N\Delta_k\delta(\theta+\phi)\gamma(-\theta)\gamma^\dagger(\phi)+\gamma(-\theta)\gamma^\dagger(\phi)\gamma^\dagger(-\phi)\gamma(\theta)
    \end{aligned},\\
    &\;\begin{aligned}
        =&(N\Delta_k)^2\delta(\theta-\phi)^2-N\Delta_k\delta(\theta-\phi)\gamma^\dagger(-\phi)\gamma(-\theta)-(N\Delta_k)^2\delta(\theta+\phi)^2+N\Delta_k\delta(\theta+\phi)\gamma^\dagger(\phi)\gamma(-\theta)\\&+N\Delta_k\delta(\theta+\phi)\gamma^\dagger(-\phi)\gamma(\theta)-\gamma^\dagger(\phi)\gamma(-\theta)\gamma^\dagger(-\phi)\gamma(\theta),
    \end{aligned}\\
    &\;\begin{aligned}
        =&(N\Delta_k)^2\delta(\theta-\phi)^2-N\Delta_k\delta(\theta-\phi)\gamma^\dagger(-\phi)\gamma(-\theta)-(N\Delta_k)^2\delta(\theta+\phi)^2+\Delta_k\delta(\theta+\phi)\gamma^\dagger(\phi)\gamma(-\theta)\\&+(N\Delta_k)\delta(\theta+\phi)\gamma^\dagger(-\phi)\gamma(\theta)-N\Delta_k\delta(\theta-\phi)\gamma^\dagger(\phi)\gamma(\theta)+\gamma^\dagger(\phi)\gamma^\dagger(-\phi)\gamma(-\theta)\gamma(\theta).
    \end{aligned}
\end{aligned}
\end{equation}
When evaluating $\bra{0_+}\mathcal{M}_\gamma\ket{0_+}$ all but two terms vanish as $\gamma$ annihilates the state when applied to $\ket{0_+}$:
\begin{equation}
\begin{aligned}
    \braket{\phi_L}{\phi_{L'}}&=(N\Delta_k)^2\mathcal{N}^2\int_{-\pi}^\pi d\theta d\phi\;\phi_L^*(\theta)\phi_{L'}(\phi)\left[\delta(\theta-\phi)^2-\delta(\theta+\phi)^2\right],\\
    &=(N\Delta_k)^2\mathcal{N}^2\int_{-\pi}^\pi d\theta \delta(0)\left[\phi_L^*(\theta)\phi_{L'}(\theta)-\phi_L^*(\theta)\phi_{L'}(-\theta)\right].
\end{aligned}
\end{equation}
The combination of the symmetric momentum interval and the exclusion principle can be used to relate $\phi_L(\theta)$ to $\phi_L(-\theta)$. 
First by just using the symmetric interval we can express the state as 
\begin{equation}
    \ket{\phi_L}=\mathcal{N}\int_{-\pi}^\pi d\theta\,\phi_L(\theta)\gamma^\dagger(\theta)\gamma^\dagger(-\theta)\ket{0_+}=\mathcal{N}\int_{-\pi}^\pi d\theta\,\phi_L(-\theta)\gamma^\dagger(-\theta)\gamma^\dagger(\theta)\ket{0_+}.
\end{equation}
However, using the anti-commuting property of the creation operators we can also express it as 
\begin{equation}
    \ket{\phi_L}=\mathcal{N}\int_{-\pi}^\pi d\theta\,\phi_L(\theta)\gamma^\dagger(\theta)\gamma^\dagger(-\theta)\ket{0_+}=-\mathcal{N}\int_{-\pi}^\pi d\theta\,\phi_L(\theta)\gamma^\dagger(-\theta)\gamma^\dagger(\theta)\ket{0_+}.
\end{equation}
As the two expression must be equal we see that $\phi_L(\theta)=-\phi_L(-\theta)$. 
The normalization thus takes the form 
\begin{equation}\label{eq:norm_mom_1}
\begin{aligned}
    \braket{\phi_L}{\phi_{L'}}&=2(N\Delta_k)^2\mathcal{N}^2\int_{-\pi}^\pi d\theta\;\delta(0)\;\phi_L^*(\theta)\phi_{L'}(\theta),\\
    &=2N^2\Delta_k\mathcal{N}^2\int_{-\pi}^\pi d\theta\;\phi_L^*(\theta)\phi_{L'}(\theta).
\end{aligned}
\end{equation}
When numerically solving the two-body problem we do it for finite $N$ in real-space. 
In that case the coefficients satisfy the relation
\begin{equation}
    \sum_{n=1}^N\phi^*_{L,n}\phi_{L',n}=\delta_{L,L'}.
\end{equation}
With this convention the integral in \cref{eq:norm_mom_1} can be evaluated
\begin{equation}
    \int_{-\pi}^\pi d\theta\;\phi_L^*(\theta)\phi_{L'}(\theta)=\int_{-\pi}^\pi d\theta\sum_{n,m}\exp\left[i\theta\left(m-n\right)\right]\phi^*_{L,n}\phi_{L',m}=2\pi\sum_n\phi^*_{L,n}\phi_{L',n}=2\pi\delta_{L,L'},
\end{equation}
giving the normalization $\mathcal{N}=1/\sqrt{4\pi\Delta_kN^2}=1/\sqrt{2(2\pi)^2N}$, such that the momentum space wave-function takes the form
\begin{equation}
    \ket{\phi_L}=\frac{1}{\sqrt{2N}}\int_{-\pi}^\pi \frac{d\theta}{2\pi}\phi_L(\theta)\gamma^\dagger(\theta)\gamma^\dagger(-\theta)\ket{0_+}.
\end{equation}
\subsection{Real-space representation}
Having found the momentum space representation of the two-fermion state it can easily be transformed to real space
\begin{equation}
\begin{aligned}
    \ket{\phi_L}&=\frac{1}{\sqrt{2N}}\sum_{n,m,m'}\int_{-\pi}^\pi \frac{d\theta}{2\pi}\exp\left[i\theta\left(n+m-m'\right)\right]\phi_{L,n}b^\dagger_{m'}b^\dagger_m\ket{0_+},\\
    &=\frac{1}{\sqrt{2N}}\sum_{n,m,m'}\delta_{n+m,m'}\phi_{L,n}b^\dagger_{m'}b^\dagger_m\ket{0_+},\\
    &=\frac{1}{\sqrt{2N}}\sum_{n,m}\phi_{L,n}b^\dagger_{m+n}b^\dagger_m\ket{0_+},\\
    \end{aligned}
\end{equation}
which is indeed a translation-invariant two-fermion state. 
The normalization of the state is given as
\begin{equation}
    \begin{aligned}
        \braket{\phi_L}{\phi_{L'}}=\frac{1}{2N}\sum_{n,m,n',m'}\phi^*_{L,n}\phi_{L',n'}\bra{0_+}b_{m}b_{m+n}b_{m'+n'}^\dagger b_{m'}^\dagger\ket{0_+}.
    \end{aligned}
\end{equation}
Evaluating the expectation value is again done using the anti-commutation relations
\begin{equation}
    \begin{aligned}
        \bra{0_+}b_{m}b_{m+n}b_{m'+n'}^\dagger b_{m'}^\dagger\ket{0_+}&=\bra{0_+}b_{m}\left(\delta_{m+n,m'+n'}-b_{m'+n'}^\dagger b_{m+n} \right)b_{m'}^\dagger\ket{0_+},\\
        &=\delta_{m+n,m'+n'}\delta_{m,m'}-\bra{0_+}b_{m}b_{m'+n'}^\dagger b_{m+n} b_{m'}^\dagger\ket{0_+},\\
        &=\delta_{m+n,m'+n'}\delta_{m,m'}-\bra{0_+}b_{m}b_{m'+n'}^\dagger \delta_{m+n,m'}\ket{0_+},\\
        &=\delta_{m+n,m'+n'}\delta_{m,m'}-\delta_{m+n,m'}\delta_{m'+n',m}.
    \end{aligned}
\end{equation}
Inserting this into the normalization 
\begin{equation}
    \begin{aligned}
        \braket{\phi_L}{\phi_{L'}}=\frac{1}{2N}\sum_{n,m}\left(\phi^*_{L,n}\phi_{L',n}-\sum_{n',m'}\phi^*_{L,n}\phi_{L',n'}\delta_{m',m+n}\delta_{n',-n}\right).
    \end{aligned}
\end{equation}
The modulo nature means that $\delta_{n,-n'}$ should be understood as $\delta_{n,N-n}$. 
As we consider the even fermion sector the boundary conditions are anti-periodic \cite{IsingBeginners}.  
Using the ABC one finds
\begin{equation}\label{eq:space_normalization}
    \begin{aligned}
        \braket{\phi_L}{\phi_{L'}}=\frac{1}{N}\sum_{n,m}\phi^*_{L,n}\phi_{L',n}=\sum_{n}\phi^*_{L,n}\phi_{L',n}=\delta_{L,L'},
    \end{aligned}
\end{equation}
which is consistent with normalization we are using.

\subsection{Coupling to FV and magnetization}
Due to $\tilde{V}$ the two-fermion states are coupled to the FV.
One can compute this coupling analytically \cite{Rutkevich1999,Wilczek2023}
\begin{equation}\label{eq:FVbub_overlap}
    \Omega_L\equiv\bra{0_+}V\ket{\phi_L}=\frac{1}{2}\sqrt{N}M J\abs{h_\parallel}\sum_{n=1}^N h_\perp^n\phi_{L,n}=\Omega_L^*.
\end{equation}
The potential is also useful to compute the average magnetization of the state through the definition of $V$
\begin{equation}
  \frac{1}{N}\left<\sum_{n=1}^N\sigma^x_n\right>=\frac{\left<V\right>}{NJ \abs{h_\parallel}}.
\end{equation}
Within the truncated Hilbert space of only the FV and a single one-bubble state we can thus write the approximate average magentization operator as 
\begin{equation}\label{eq:singleBody_magOP_0}
    m_{avg}= M\dyad{0_+} +\frac{1}{NJ \abs{h_\parallel}}\sum_{L=1}^N\Omega_L\left(\dyad{0_+}{\phi_L}+\dyad{\phi_L}{0_+}\right)+\frac{1}{N J\abs{h_\parallel}}\sum_{L,L'=1}^N\tilde{\lambda}_{L,L'}\dyad{\phi_L}{\phi_{L'}},
\end{equation}
where we have defined
\begin{equation}
\bra{\phi_L}V\ket{\phi_{L'}}\approx\bra{\phi_L}V_0\ket{\phi_{L'}}=\tilde{\lambda}_{L,L'}.
\end{equation}

The overlap $\tilde{\lambda}_{L,L'}$ is straight-forward to compute as $V_0$ is diagonal in the real-space representation \cite{Rutkevich1999} and the overlaps takes the form
\begin{equation}\label{eq:lambda_tilde}
\begin{aligned}
    \tilde{\lambda}_{L,L'}=&J\abs{h_\parallel} MN\sum_{n=1}^N\phi_{L,n}^*\phi_{L',n}\left(1-\frac{2n}{N}\right),\\=&J\abs{h_\parallel} MN\sum_{n=1}^N\phi_{L,n}\phi_{L',n}\left(1-\frac{2n}{N}\right),\\=&J\abs{h_\parallel} MN\delta_{L,L'}-J\abs{h_\parallel} MN\sum_{n=1}^N\phi_{L,n}\phi_{L',n}\frac{2n}{N},
\end{aligned}
\end{equation}
where we used the fact that the spatial coefficients are real making $\tilde{\lambda}_{L,L'}$ real and symmetric. 
Using the form found for $\tilde{\lambda}_{L,L'}$ in the magnetization \cref{eq:singleBody_magOP_0} one notices that the constant terms can be combined into an identity
\begin{equation}\label{eq:singleBody_magOP}
    m_{avg}= \mathds{1}\, M+\frac{1}{N J\abs{h_\parallel}}\sum_{L=1}^N\Omega_L\left(\dyad{0_+}{\phi_L}+\dyad{\phi_L}{0_+}\right)+\frac{1}{NJ \abs{h_\parallel}}\sum_{L,L'=1}^N\lambda_{L,L'}\dyad{\phi_L}{\phi_{L'}},
\end{equation}
with 
\begin{equation}\label{eq:lambda}
\lambda_{L,L'}=-J\abs{h_\parallel} 2M\sum_{n=1}^Nn\phi_{L,n}\phi_{L',n}.
\end{equation}

\section{Many-body theory for translation-invariant bubbles}\label{sec:CBT}
As the system is translation-invariant and infinitely large a single bubble does not affect the magnetization of the system. 
This is clearly seen by $\lim_{N\to\infty}\lambda_{L,L'}/N=0$ and
$\lim_{N\to\infty}\Omega_{L}/N=0$. 
This means that a theory with only a single bubble can only be a good description when the system is described by tiny fluctuations on top of the FV \footnote{As in the case for \cite{Wilczek2023}}. 
Otherwise it is necessary to use a many-body description which allows for a finite bubble-density in the thermodynamic limit. 

The simplest conceivable many-theory is based on the infinite size of the system and the fact that the one-bubble states $\ket{\phi_L}$ consists of superpositions of bubbles with finite sizes. 
For low enough densities one thus expects that the state can be approximated as multiple non-interacting bubbles.
Each bubble consists of two fermions, so as long as the bubbles do not interact with each other it should be valid to think of the bubbles as non-interacting bosons.
This idea belongs in the broader scope of methods known as cobosonization \cite{Tichy2014}. 
Within this method we define a creation operator for the $L$'th bubble state
\begin{equation}
    d^\dagger_L=\frac{1}{\sqrt{2N}}\int_{-\pi}^\pi\frac{d\theta}{2\pi}\phi_L(\theta)\gamma^\dagger(\theta)\gamma^\dagger(-\theta),
\end{equation}
The anti-commutation relations of the fermions in \cref{eq:fermionAC_finite} directly leads to
\begin{equation}
\left[d^\dagger_L,d^\dagger_{L'}\right]=\Big[d_L,d_{L'}\Big]=0,
\end{equation}
while
\begin{equation}\label{eq:d_commutationRelation}
    \left[d_L,d^\dagger_{L'}\right]=\frac{1}{2N}\int_{-\pi}^\pi\frac{d\theta d\theta'}{(2\pi)^2}\phi_L^*(\theta)\phi_{L'}(\theta')\left[\gamma(-\theta)\gamma(\theta),\gamma^\dagger(\theta')\gamma^\dagger(-\theta')\right].
\end{equation}
We already did the cumbersome part of the calculation of the commutation relation in \cref{eq:Mgamma}
\begin{equation}
\begin{aligned}
    \left[\gamma(-\theta)\gamma(\theta),\gamma^\dagger(\theta')\gamma^\dagger(-\theta')\right]&=M_\gamma(\theta,\theta')-\gamma^\dagger(\theta')\gamma^\dagger(-\theta')\gamma(-\theta)\gamma(\theta),\\
    &\;\begin{aligned}
        =&(N\Delta_k)^2\delta(\theta-\phi)^2-N\Delta_k\delta(\theta-\phi)\gamma^\dagger(-\phi)\gamma(-\theta)-(N\Delta_k)^2\delta(\theta+\phi)^2+N\Delta_k\delta(\theta+\phi)\gamma^\dagger(\phi)\gamma(-\theta)\\&+N\Delta_k\delta(\theta+\phi)\gamma^\dagger(-\phi)\gamma(\theta)-N\Delta_k\delta(\theta-\phi)\gamma^\dagger(\phi)\gamma(\theta).
    \end{aligned}
\end{aligned}
\end{equation}
Inserting this into \cref{eq:d_commutationRelation} one finds
\begin{equation}
\begin{aligned}\label{eq:TI_Commutation}
    \left[d_L,d^\dagger_{L'}\right]=&\frac{1}{2N}\int_{-\pi}^\pi\frac{d\theta}{(2\pi)^2}\Big[(N\Delta_k)^2\delta(0)\phi_L^*(\theta)\phi_{L'}(\theta)-(N\Delta_k)^2\delta(0)\phi_L^*(\theta)\phi_{L'}(-\theta)-N\Delta_k\phi_L^*(\theta)\phi_{L'}(\theta)\gamma^\dagger(-\theta)\gamma(-\theta)\\&\hspace{24mm}+N\Delta_k\phi_L^*(\theta)\phi_{L'}(-\theta)\gamma^\dagger(-\theta)\gamma(-\theta)-N\Delta_k\phi_L^*(\theta)\phi_{L'}(\theta)\gamma^\dagger(\theta)\gamma(\theta)+N\Delta_k\phi_L^*(\theta)\phi_{L'}(-\theta)\gamma^\dagger(\theta)\gamma(\theta)\Big],\\
    =&\frac{\Delta_k}{2}\int_{-\pi}^\pi\frac{d\theta}{(2\pi)^2}\Big[N\phi_L^*(\theta)\phi_{L'}(\theta)-N\phi_L^*(\theta)\phi_{L'}(-\theta)-\phi_L^*(\theta)\phi_{L'}(\theta)\gamma^\dagger(-\theta)\gamma(-\theta)\\&\hspace{24mm}+\phi_L^*(\theta)\phi_{L'}(-\theta)\gamma^\dagger(-\theta)\gamma(-\theta)-\phi_L^*(\theta)\phi_{L'}(\theta)\gamma^\dagger(\theta)\gamma(\theta)+\phi_L^*(\theta)\phi_{L'}(-\theta)\gamma^\dagger(\theta)\gamma(\theta)\Big],\\
    =&\delta_{L,L'}-\frac{2}{N}\int_{-\pi}^\pi \frac{d\theta}{2\pi}\phi_L^*(\theta)\phi_{L'}(\theta)\gamma^\dagger(\theta)\gamma(\theta),
\end{aligned}
\end{equation}
where the anti-symmetry of $\phi_L(\theta)$ have been exploited. 
This result clearly shows that bosonic commutation relations emerge when only one bubble is present in the system. 

In the real-space representation of the bubble-operator the results is
\begin{equation}
    \left[d_L,d^\dagger_{L'}\right]=\delta_{L,L'}-\frac{2}{N}\sum_{n,m,m'=1}^N\phi_{L,n}^*\phi_{L',m}b^\dagger_{m-n+m'}b_{m'}.
\end{equation}
Considering translation-invariance (and thereby doing the sum over $m'$) one finds
\begin{equation}\begin{aligned}
\left[d_L,d^\dagger_{L'}\right]&=\delta_{L,L'}-2\sum_{n,m}^N\phi_{L,n}^*\phi_{L',m}b^\dagger_{m-n}b_0.
\end{aligned}
\end{equation}

One notices that in the $h_\perp\to0$ case the fermion wave functions becomes strongly localized $\phi_L,n\approx\delta_{L,n}$.
In this case the perturbation to the bosonic commutator becomes 
\begin{equation}
\lim_{h_\perp\to0}\left[d_L,d^\dagger_{L'}\right]=\delta_{L,L'}-2 b^\dagger_{L-L'}b_0,
\end{equation}
which is always unity for $L=L'$ but is related to the fermion two-point correlation function for $L\neq L'$. 
\subsection{Coherent boson theory}
We will now assume that the density of bubbles is small enough that the violation of the bosonic commutation relations in \cref{eq:TI_Commutation} can be neglected. 
Under this assumption the state with $n$ bubbles of type $L$ and $m$ bubbles of type $L'$ is given as 
\begin{equation}
    \ket{n_L,m_{L'}}=\frac{1}{\sqrt{n!m!}}\left(d_L^\dagger\right)^n\left(d_{L'}^\dagger\right)^m\ket{0_+}.
\end{equation}
The Hamiltonian contains the single bubble energies and their coupling to the FV
\begin{equation}
H=\sum_{L=1}^NE_Ld^\dagger_Ld_L+\Omega_L\left(d_L+d^\dagger_L\right).
\end{equation}
The non-interacting nature of the bosons means that we can diagonialize the Hamiltonian using a multi-mode displacement operator
\begin{equation}
    D = \bigotimes_LD_L(\alpha_L),
\end{equation}
with the single-mode displacement operator being defined as 
\begin{equation}
    D_L(\alpha)=\exp\left(\alpha d_L^\dagger-\alpha^* d_L\right).
\end{equation}
This operator is unitary with 
\begin{equation}
D_L^\dagger(\alpha)=D_L^{-1}(\alpha)=D_L(-\alpha),    
\end{equation}
and its action on the annihilation and creation operators are simple shifts
\begin{equation}
\begin{aligned}
    D_L^\dagger(\alpha)d_LD_L(\alpha)&=d_L+\alpha,\\
    D_L^\dagger(\alpha)d_L D_L(\alpha)&=d_L^\dagger+\alpha^*.
\end{aligned}
\end{equation}
When the displacement operator is applied to the vacuum state it generates a coherent state
\begin{equation}
    D_L(\alpha_L)\ket{0_+}=\exp\left(-\frac{1}{2}\abs{\alpha_L}^2\right)\sum_{n=0}^N\frac{\alpha_L^n}{\sqrt{n!}}\ket{n_L}=\ket{\alpha_L}.
\end{equation}
As the coherent states constitute an over-complete basis the overlap of two coherent states is finite
\begin{equation}\label{eq:overlap_coh}
    \abs{\ip{\alpha_L}{\beta_L}}^2=\exp\left(-\abs{\alpha_L-\beta_L}^2\right).
\end{equation}
Applying the multi-mode displacement operator to the Hamiltonian one finds 
\begin{equation}
    \begin{aligned}
        \tilde{H}&=D^\dagger HD,\\
        &=\sum_L E_L\left(d^\dagger_L+\alpha_L^*\right)\Big(d_L+\alpha_L\Big)+\Omega_L\left(d^\dagger_L+d_L+2\text{Re}(\alpha_L)\right),\\
        &=\sum_L E_L d^\dagger_Ld_L+E_L\abs{\alpha_L}^2+2\text{Re}(\alpha_L)\Omega_L+\left(\Omega_L+E_L\alpha_L^*\right)d_L+\left(\Omega_L+E_L\alpha_L\right)d_L^\dagger,
    \end{aligned}
\end{equation}
where we will use the tilde to indicate that we are in the displaced basis. 
The linear terms can be removed by choosing $\alpha_L=-\Omega_L/E_L$, which makes the Hamiltonian diagonal
\begin{equation}
    \tilde{H}=\sum_L E_L d^\dagger_L d_L-\frac{\Omega_L^2}{E_L}.
\end{equation}
One observes that this Hamiltonian is a simple harmonic oscillator where each mode acquires a shift. 
As the modes do not interact this shift just leads to an overall phase of the wave-function $\sum_L\Omega_L^2/E_L=\chi$. 
Any time evolved state can therefore simply be represented as 
\begin{equation}
    \ket{\tilde{\psi}(t)}=e^{it \chi}\sum_{\{n_L\}}c_{\{n_L\}}\exp\left(-i\sum_LE_Ln_L t\right)\ket{n_1,n_2,...,n_N}=e^{it \chi}\sum_{\{n_L\}}c_{\{n_L\}}\bigotimes_L\exp\left(-iE_Ln_L t\right)\ket{n_L}.
    \end{equation}
For our purpose we are interested in time evolving a specific state, namely, the false vacuum state. 
Transforming the FV to the diagonal basis is straightforward
\begin{equation}
   \begin{aligned}
       \ket{\tilde{\psi}(0)}=D^\dagger\ket{0_+}=\bigotimes_LD_L(\Omega_L/E_L)\ket{0_+}=\bigotimes_L\ket{\Omega_L/E_L}=\bigotimes_L\exp\left[-\frac{1}{2}\left(\frac{\Omega_L}{E_L}\right)^2\right]\sum_{n=0}^N\frac{\left(\frac{\Omega_L}{E_L}\right)^n}{\sqrt{n!}}\ket{n_L},
   \end{aligned} 
\end{equation}
The coefficients in the wave-function expansion now takes the form 
\begin{equation}
    \ip{\tilde{\psi}(0)}{n1,n2,...,n_N}=\prod_L\exp\left[-\frac{1}{2}\left(\frac{\Omega_L}{E_L}\right)^2\right]\frac{\left(\frac{\Omega_L}{E_L}\right)^{n_L}}{\sqrt{n_L!}}.
\end{equation}
As the these coefficients are just a product over the modes the entire time-evolved state is a product state for all times
\begin{equation}\label{eq:timeDep_state}
\begin{aligned}
    \ket{\tilde{\psi}(t)}&=e^{it\chi}\bigotimes_L\exp\left[-\frac{1}{2}\left(\frac{\Omega_L}{E_L}\right)^2\right]\sum_{\{n_L\}}\frac{\left(\frac{\Omega_L}{E_L}\right)^{n_L}}{\sqrt{n_L!}}\exp\left(-iE_Ln_L t\right)\ket{n_L},\\&=e^{it\chi}\bigotimes_L\exp\left[-\frac{1}{2}\left(\frac{\Omega_L}{E_L}\right)^2\right]\sum_{\{n_L\}}\frac{\left(\frac{\Omega_L}{E_L}e^{-iE_L t}\right)^{n_L}}{\sqrt{n_L!}}\ket{n_L},\\&=e^{it\chi}\bigotimes_L\ket{\frac{\Omega_Le^{-iE_L t}}{E_L}},
    \end{aligned}
\end{equation}
which is just a product state of coherent states. 
Due to the unitarity of the displacement operator the state is also trivially normalized for all times. 

\subsubsection{Dynamics of excitations}
If one considers the number of bubbles in the $L$'th state then this is given by 
\begin{equation}
\begin{aligned}
    \bra{\psi(t)}d_L^\dagger d_L\ket{\psi(t)}&=\bra{\tilde{\psi}(t)}D^\dagger d_L^\dagger D D^\dagger d_LD\ket{\tilde{\psi}(t)},\\&=\bra{\tilde{\psi}(t)} \left(d_L^\dagger-\frac{\Omega_L}{E_L}\right) \left(d_L-\frac{\Omega_L}{E_L}\right)\ket{\tilde{\psi}(t)},\\
    &=\bra{\tilde{\psi}(t)} \left(d^\dagger_Ld_L+\left(\frac{\Omega_L}{E_L}\right)^2-d_L^\dagger \frac{\Omega_L}{E_L}-d_L \frac{\Omega_L}{E_L}\right)\ket{\tilde{\psi}(t)},\\
    &=\left(\frac{\Omega_L}{E_L}\right)^2\left(2-e^{iE_Lt}-e^{-iE_Lt}\right),\\
    &=2\left(\frac{\Omega_L}{E_L}\right)^2\left[1-\cos\left(E_Lt\right)\right],\\
    &=\left(\frac{2\Omega_L}{E_L}\right)^2\sin^2\left(E_Lt/2\right),
    \end{aligned}
\end{equation}
which means that the system initially has no occupation and is therefore consistent with the initial state used. 
With this result our prediction is that the dynamics of the $L$'th bubble has a time-scale directly set by $1/E_L$ but that its "importance"/magnitude in the dynamics is set by $\left(\frac{\Omega_L}{E_L}\right)^2$. 
As the system is infinite the relevant quantity is not the number of bubbles but instead their density 
\begin{equation}\label{eq:NL}
    \mathcal{N}_{L}=\frac{\bra{\psi(t)}d_L^\dagger d_L\ket{\psi(t)}}{N}=\frac{1}{N}\left(\frac{2\Omega_L}{E_L}\right)^2\sin^2\left(E_Lt/2\right).
\end{equation}
Since $\Omega_L\propto \sqrt{N}$ as seen in \cref{eq:FVbub_overlap} and $E_L$ is an intensive quantity, the density of the $L$'th bubble becomes intensive and therefore well-defined in the thermodynamic limit. 
This observable describes the average number of bubbles of species $L$ at a single site. 
For the case of a resonant bubble, $E_r\to 0$ allowing us to expand the sine
\begin{equation}
    N_{r}=\frac{\Omega_r^2 t^2}{N},
\end{equation}
giving the resonant physics a time scale of 
\begin{equation}
    T_{r}=\frac{1}{2 JM \abs{h_\parallel}\sum_{n=1}^N h_\perp^n\phi_{r,n}}.
\end{equation}

\subsubsection{Average magnetization}
To compare the results of the CBT with MPS calculations, we wish to compute an approximation to the average magnetization within the CBT.
To compute the magnetization we can directly promote the single-body average magnetization operator in \cref{eq:singleBody_magOP} to a many body-operator
\begin{equation}
    m_{avg} = M +\frac{1}{NJ \abs{h_\parallel}}\sum_{L=1}^N\Omega_L\left(d_L+d^\dagger_L\right)+\frac{1}{N J\abs{h_\parallel}}\sum_{L,L'=1}^N\lambda_{L,L'}d_L^\dagger d_{L'},
\end{equation} 
where we remind the reader that there is an additional flat-band approximation in $\lambda_{L,L'}$.
Using the same procedure as for the bubble occupation we transform $m_{avg}$ to the displaced basis
\begin{equation}
\begin{aligned}
    \tilde{m}_{avg}&=D^\dagger m_{avg}D,\\
    &=M+\frac{1}{NJ\abs{h_\parallel}}\sum_L\Omega_L
    \left(d_L+d^\dagger_L-2\frac{\Omega_L}{E_L}\right)+\frac{1}{NJ\abs{h_\parallel}}\sum_{L,L'}\lambda_{L,L'}
    \bigg(d^\dagger_L-\frac{\Omega_L}{E_L}\bigg)\bigg(d_{L'}-\frac{\Omega_{L'}}{E_{L'}}\bigg),\\
    &=M+\frac{1}{NJ\abs{h_\parallel}}\sum_L\Omega_L
    \left(d_L+d^\dagger_L-2\frac{\Omega_L}{E_L}\right)+\frac{1}{NJ\abs{h_\parallel}}\sum_{L,L'}\lambda_{L,L'}
    \Bigg[d^\dagger_L d_{L'}-\frac{\Omega_L}{E_L}d_{L'}\\&\hspace{95mm}-\frac{\Omega_{L'}}{E_{L'}}d^\dagger_L+\frac{\Omega_L\Omega_{L'}}{E_L E_{L'}}\Bigg],\\
    &=M+G_\Omega+G_\lambda.
\end{aligned}
\end{equation}
We can now compute overlaps with the time-dependent state in \cref{eq:timeDep_state} of the two different terms. 
The first contribution arises from the coupling between the false vacuum and one-bubble states
\begin{equation}\label{eq:mag_crossTerms}
\begin{aligned}
    \langle G_\Omega\rangle(t)&=\bra{\psi(t)}G_\Omega\ket{\psi(t)},\\
    &=\frac{1}{N J\abs{h_\parallel}}\sum_L\Omega_L\left[\frac{\Omega_L e^{-it E_L}}{E_L}+\frac{\Omega_L e^{it E_L}}{E_L}-2\frac{\Omega_L}{E_L}\right],\\
    &=\frac{1}{N J\abs{h_\parallel}}\sum_L\frac{\Omega_L^2}{E_L}\left[e^{-it E_L}+e^{it E_L}-2\right],\\
    &=\frac{2}{N J\abs{h_\parallel}}\sum_L\frac{\Omega_L^2}{E_L}\left[\cos\left(E_L t\right)-1\right].\\
\end{aligned}
\end{equation}
This term is seen to be intensive and consistent with our initial state as the entire contribution vanishes at $t=0$. 

The second term is related to the magnetization of a bubble state 
\begin{equation}\label{eq:T_lambda}
\begin{aligned}
    \langle G_\lambda\rangle(t)&=\bra{\psi(t)}G_\lambda\ket{\psi(t)},\\
    &=\frac{1}{N J\abs{h_\parallel}}\sum_{L,L'}\lambda_{L,L'}\frac{\Omega_L\Omega_{L'}}{E_L E_{L'}}\Big(e^{i(E_L-E_{L'})t}-e^{-iE_{L'}t}-e^{iE_L t}+1\Big),\\
    &=\frac{1}{2N J\abs{h_\parallel}}\sum_{L,L'}\lambda_{L,L'}\frac{\Omega_L\Omega_{L'}}{E_L E_{L'}}\Big(e^{i(E_L-E_{L'})t}+e^{-i(E_L-E_{L'})t}-e^{-iE_{L'}t}-e^{iE_{L'}t}-e^{iE_L t}-e^{-iE_L t}+2\Big),\\
    &=\frac{1}{N J\abs{h_\parallel}}\sum_{L,L'}\lambda_{L,L'}\frac{\Omega_L\Omega_{L'}}{E_L E_{L'}}\Big(\cos\left\{(E_L-E_{L'})t\right\}-2\cos\left(E_{L}t\right)+1\Big),\\
\end{aligned}
\end{equation}
where in the third line we used the symmetric property of $\lambda_{L,L'}$ seen in \cref{eq:lambda}. 
As for $\langle G_\Omega\rangle$ also $\langle G_\lambda\rangle$ satisfies the consistency check that it vanishes at $t=0$. 
One notices that the extensive property of $\Omega_L$ is canceled and since $\lambda_{L,L'}$, in \cref{eq:lambda}, is intensive the average magnetization is intensive as it should be. 
After some initial time one expects that the physics is dominated by the resonant bubble. Assuming that an almost resonant bubble exists in the system such that we can expand the cosines the slow envelope of the magnetization grows quadratically
\begin{equation}
    \lim_{E_r\to0}\langle m_{avg}\rangle(t)=M-\frac{\Omega_r^2 t^2}{N J\abs{h_\parallel}}\left(E_R+\lambda_r\right)=M-\frac{\lambda_r\Omega_r^2 t^2}{N J\abs{h_\parallel}}.
\end{equation}

\subsubsection{Dynamics of bubbles}
The density of bubbles of size $n$ is straight-forward to compute within the single-bubble theory 
\begin{equation}\
    P_n = \frac{1}{N}\abs{\bra{0_+}\sum_m b_mb_{n+m}\ket{\psi(t)}}^2
\end{equation}
as the operators $b_n$ action on $\ket{\psi}$ is well-understood.
In the many-bubble theory the wave-function has the form 
\begin{equation}
    \ket{\psi}(t)=\sum_{m,L} c_{m,L}\left(d_L^\dagger\right)^m\ket{0_+}.
\end{equation}
The action of $b_n$ on the coherent boson states is highly non-trivial and we can therefore not directly compute $P_n$.
However, if we neglect the quantum cross-terms then we can write an approximation for the overlap between 
states with fermions a distance $n$ apart and our coherent states given by
\begin{equation}
    \braket{n}{\psi} = \frac{1}{\sqrt{N}}\sum_L \langle d_L^\dagger\rangle \phi_L(n).
\end{equation}
Within this approximation $P_n$ is given by
\begin{equation}\label{eq:Pn}
\begin{aligned}
    P_n&=\frac{1}{N}\sum_{L,L'} \langle d_L^\dagger\rangle \langle d_{L'}\rangle \phi_L(n)\phi_{L'}^*(n),\\
    &= \sum_{L,L'}\alpha_{L,L'}(n)\Big\{\cos\left[t(E_L-E_{L'}|)\right]-2\cos(t E_L)+1\Big\},
\end{aligned}
\end{equation}
where
\begin{equation}
    \alpha_{L,L'}(n)=\frac{1}{N}\phi_L(n)\phi_{L'}^*(n)\frac{\Omega_L \Omega_{L'}}{E_L E_{L'}}.
\end{equation}
As a sanity check we can compute the total density of bubbles in the system
\begin{equation}
    \begin{aligned}
        \sum_nP_n&=\frac{1}{N}\sum_{L,L',n} \langle d_L^\dagger\rangle \langle d_{L'}\rangle \phi_L(n)\phi_{L'}^*(n),\\
        &=\frac{1}{N}\sum_{L,L'} \langle d_L^\dagger\rangle \langle d_{L'}\rangle \delta_{L,L'},\\
        &=\frac{1}{N}\sum_L \langle d_L^\dagger d_L\rangle,\\
        &=\mathcal{N},
    \end{aligned}
\end{equation}
 with the excitation density defined in \cref{eq:NL}. 
 So the number-density of spatial bubbles is equivalent to the total number-density of bosonic excitation as one would expect from our simple non-interacting theory. 

To show that some care has to be taken with our approximation of $P_n$ we can use it to compute the magnetization. 
Within our approximate picture and with only a small excitation density, the magnetization should be related to the density of TV domains through
\begin{equation}
    m(t)\approx M\left[1-2\rho(t)\right]=M\left[1-2\sum_n n P_n(t)\right].
\end{equation}
Writing out the last term
\begin{equation}
\begin{aligned}
    -2M \sum_n n P_n(t)&=-2M \sum_{n,L,L'} n\alpha_{L,L'}(n) F(t),\\
    &=-2M \sum_{n,L,L'} \frac{n\phi_L(n)\phi_{L'}^*(n)}{N}\frac{\Omega_L \Omega_{L'}}{E_L E_{L'}} F(t),\\
\end{aligned} 
\end{equation}
 where $F(t)$ is the time-dependent function in the curly brackets in \cref{eq:Pn}.
 Writing out the $\lambda$-contribution to the magnetization in \cref{eq:T_lambda} one finds
 \begin{equation}
 \begin{aligned}
     \langle G_\lambda\rangle(t)=\sum_{L,L'}\frac{-2 M n \phi_L(n)\phi_{L'}^*(n)}{N}\frac{\Omega_L\Omega_{L'}}{E_L E_{L'}}F(t)=-2M \sum_n n P_n(t).
 \end{aligned}
 \end{equation}
 This means that using $P_n$ to compute the magnetization will be off as the quantum cross-terms from $G_\Omega$ in \cref{eq:mag_crossTerms} are missing. 
So quantities computed with $P_n$ generically includes additional approximations on top of the ones already present in CBT. 
\begin{figure}
    \centering
\includegraphics[width=.5\linewidth]{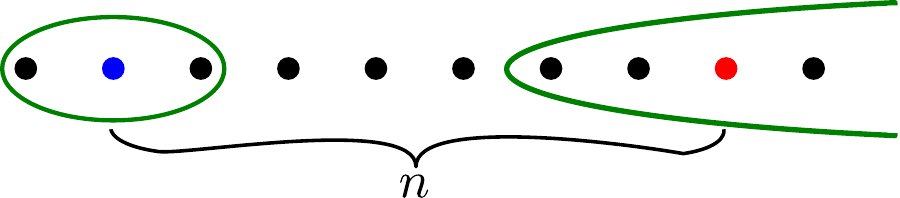}
    \caption{Sketch illustrating how to compute the correlation function. The green ovals represent TV bubbles.}
    \label{fig:corr}
\end{figure}
\subsection{spin-spin correlation function}
To understand how all spatial structure in the fermions translate into dynamics in the spin chain we consider approximating the spin-spin correlation function given by
\begin{equation}
    C_{n}(t)=\frac{1}{N}\sum_{j=1}^N\left(\langle\sigma^x_{n+j}\sigma^x_j\rangle-\langle\sigma^x_j\rangle^2\right).
\end{equation}
To approximate this we first want to compute the probability, $Q_n$, of two spins having opposite magnetization when being separated by $n$ sites. 
So specifically we want to compute the probability that the red and blue site in \cref{fig:corr} have opposite magnetization. 
Consistent with our assumption that the excitation is small we consider the probability in the case when only one bubble is present within this region.
There are two different scenarios that must be accounted for. 
The first is illustrated around the red site in \cref{fig:corr} (ignore bubble around blue site). 
In this scenario the bubble size $l_B$ is large than the separation between the sites: $l_B>n$. 
In this case there are $n$ different locations for the bubble such that the red site is covered but the blue site is not. 
The opposite regime of $l_B<n$ is illustrated around the blue site (ignore the previously discussed bubble around the red site). 
In this case there are $l_B$ different locations where the blue site is covered and thus gives rise to opposite magnetization of the two colored sites. 
Putting this together we can write the probability of the two spins having opposite magnetization as
\begin{equation}
    Q_n(t)=2\sum_l \textrm{min}(n,l) P_l(t),
\end{equation}
where the factor of two arises from the fact that we also have to included the processes where the two sites are swapped (large bubble from the left and small bubble to right). 
With this object we are able to compute the total spin-spin correlation function as a sum of two contributions.
The first is the probability of the two spins pointing in the same direction and the second is the probability of them being opposite
\begin{equation}
\begin{aligned}
    \mathcal{C}_n(t)&=\frac{1}{N}\sum_{j=1}^N\langle\sigma^x_{n+j}\sigma^x_j\rangle(t),\\&=M^2\left[1-Q_n(t)\right]+M^2\left[-Q_n(t)\right],\\
    &=M^2\left[1-2Q_n(t)\right],\\
    &=M^2\left[1-4\sum_l \textrm{min}(n,l) P_l(t)\right].
\end{aligned}
\end{equation}
To compute the disconnected contribution we consider the limit of $\lim_{n\to\infty}$
\begin{equation}
    \begin{aligned}
        \lim_{n\to\infty}\mathcal{C}_n(t)&=\frac{1}{N}\sum_{j}\langle\sigma^x_n\rangle\langle\sigma^x_j\rangle,\\
        &=\frac{1}{N}\sum_{j}\langle\sigma^x_j\rangle^2,\\
        &=M^2\left[1-4\sum_l l P_l(t)\right],\\
        &=M^2\left[1-4\rho(t)\right],
    \end{aligned}
\end{equation}
where we have exploited the translation invariance of the system.
With these results we can approximate the connected spin-spin correlation function as
\begin{equation}
    C_n(t)=4M^2\sum_{l=n+1}^N (l-n) P_l(t).
\end{equation}
The approximation has the simple intuitive structure that only bubbles larger than the distance between the sites contribute to the connected correlations. 

Lastly we remark that for both the magnetization and the correlation function we have neglected the delocalized nature of the domain walls which is only valid if the relevant fermion bubbles are much larger that the domain wall spreading in \cref{eq:W}. 
For the considered parameters in the main text this is the case as for the rigid parameters $W_\rho\approx0.26$ where the resonant bubble is of size $4$, while for the expandable regime $W_\chi\approx3.46$ where the bubbles extend up to more than a hundred lattice sites (see plot of $\abs{\phi_{r}(n)}^2$ in main text).
\bibliography{bib.bib}
\end{document}
